# Supplementary material for: DeepPhys: Video-Based Physiological Measurement Using Convolutional Attention Networks
Source: arXiv:1805.07888 ancillary file (2018-08-07)
Supplement: Supplementary file 1 [file Supplementary_Material_III.pdf]

# DeepPhys: Video-Based Physiological Measurement Using Convolutional Attention Networks

## *Supplemental Material III*

Weixuan Chen<sup>1</sup> and Daniel McDuff<sup>2</sup>

<sup>1</sup>Massachusetts Institute of Technology, Cambridge, Massachusetts

<sup>2</sup>Microsoft Research, Redmond, Washington

March 2018

## Implementation Details of Previous Methods

For comparison with our proposed approach, we implemented several state-of-the-art methods of video-based physiological measurement as faithfully as possible based on their original papers. Below are some details we feel worth mentioning in our implementations:

**McDuff et al. [7]:** The OpenFace [2] landmark tracker was used for facial region of interest segmentation. The whole face was segmented along the chin contour and around the top of the forehead. The pixels in the region of interest were spatially averaged to obtain the observation signals. The detrending parameter  $\lambda$  was fixed at 1000 and the bandpass filter thresholds at [0.7, 2.5] Hz, or [42, 150] BPM. The Jade implementation of ICA was used for signal decomposition. The blood volume pulse was selected as the source signal with the greatest power in the range [0.7, 2.5] Hz.

**Estepp et al. [5]:** The implementation was identical to that described above except the whole frame was used in the spatial averaging step (i.e., no face segmentation was applied).

**Balakrishnan et al. [1]:** The algorithm assumes that a normal adult’s resting pulse rate falls within [0.75, 2] Hz, or [45, 120] beats/min, so it applied a 5th order Butterworth filter with a passband of [0.75, 5] Hz to its output signals. However, some of the subjects in our four datasets have a slightly lower heart rate than 45 beats/min, so we used a passband of [0.7, 5] Hz instead in the filter.

**De Haan et al. [6]:** To minimize the impact of unintended motion, 500 consecutive pictures (25 seconds in time length) exhibiting the smallest amount of inter-frame motion were selected from their 60-second test windows to represent the whole sequences. However, in our experiments the test windows are 30 seconds in length. As selecting 25 seconds from 30-second windows made nearly no difference to the results, we omitted this step. Also, the paper says it applies a simple skin selection process after face detection, but does not give any details about the process. We used a widely adopted method [3] for skin selection in our implementation.

Table 1: Root mean square error (RMSE) and Pearson’s correlation coefficient ( $r$ ) of heart rate and breathing rate measurement for RGB Video I. Participant dependent (p.-dep.) and participant independent results are shown, as are task independent results for the six tasks with varying levels of head rotation

| <b>HEART RATE</b>       |  | Root Mean Square Error / BPM |      |      |      |      |      |      | Pearson’s Correlation Coefficient |      |      |       |       |       |      |
|-------------------------|--|------------------------------|------|------|------|------|------|------|-----------------------------------|------|------|-------|-------|-------|------|
| Methods                 |  | 1                            | 2    | 3    | 4    | 5    | 6    | Avg. | 1                                 | 2    | 3    | 4     | 5     | 6     | Avg. |
| Estepp et al. [5]       |  | 7.15                         | 8.52 | 7.59 | 11.5 | 18.0 | 17.4 | 12.5 | .802                              | .761 | .807 | .676  | .312  | .235  | .564 |
| McDuff et al. [7]       |  | 2.17                         | 4.00 | 4.77 | 9.24 | 10.5 | 16.3 | 9.18 | .981                              | .946 | .919 | .754  | .692  | .339  | .741 |
| Balakrishnan et al. [1] |  | 10.6                         | 12.0 | 18.5 | 22.3 | 23.3 | 18.5 | 18.2 | .855                              | .838 | .710 | .738  | .715  | .818  | .729 |
| De Haan et al. [6]      |  | 10.2                         | 9.83 | 10.1 | 11.2 | 15.4 | 17.9 | 12.8 | .669                              | .726 | .712 | .681  | .481  | .392  | .592 |
| Wang et al. [10]        |  | 3.03                         | 2.97 | 4.38 | 4.83 | 5.06 | 10.7 | 5.78 | .964                              | .971 | .933 | .925  | .917  | .709  | .891 |
| Tulyakov et al. [9]     |  | 3.89                         | 4.57 | 19.1 | 24.0 | 21.0 | 26.4 | 16.5 | .945                              | .931 | .070 | .163  | .236  | -.004 | .390 |
| <b>OURS: Part. Dep.</b> |  |                              |      |      |      |      |      |      |                                   |      |      |       |       |       |      |
| Motion-only CNN         |  | 2.30                         | 2.43 | 3.71 | 4.33 | 6.09 | 7.75 | 4.44 | .979                              | .980 | .949 | .938  | .872  | .810  | .921 |
| Stacked CNN             |  | 2.75                         | 2.76 | 3.59 | 3.76 | 5.55 | 7.48 | 4.31 | .970                              | .974 | .952 | .954  | .893  | .824  | .928 |
| CAN                     |  | 2.65                         | 2.45 | 3.26 | 4.09 | 6.33 | 4.95 | 3.96 | .973                              | .979 | .960 | .945  | .863  | .919  | .940 |
| <b>OURS: Part. Ind.</b> |  |                              |      |      |      |      |      |      |                                   |      |      |       |       |       |      |
| Motion-only CNN         |  | 2.39                         | 2.81 | 3.89 | 4.67 | 8.50 | 12.2 | 5.75 | .977                              | .973 | .944 | .929  | .772  | .598  | .866 |
| Stacked CNN             |  | 1.98                         | 4.12 | 3.93 | 4.19 | 6.36 | 12.3 | 5.47 | .984                              | .943 | .942 | .942  | .866  | .578  | .876 |
| CAN                     |  | 2.46                         | 2.88 | 3.63 | 4.47 | 6.69 | 11.4 | 5.25 | .976                              | .972 | .951 | .934  | .851  | .638  | .887 |
| CAN (task 1)            |  | 2.46                         | 9.34 | 9.97 | 11.3 | 14.0 | 17.6 | 10.8 | .976                              | .746 | .677 | .637  | .480  | .162  | .613 |
| CAN (task 2)            |  | 1.96                         | 2.82 | 4.48 | 7.37 | 13.5 | 16.8 | 7.82 | .985                              | .994 | .927 | .833  | .505  | .247  | .748 |
| CAN (task 3)            |  | 2.44                         | 2.62 | 3.63 | 4.86 | 7.73 | 14.4 | 5.95 | .977                              | .976 | .951 | .921  | .803  | .459  | .848 |
| CAN (task 4)            |  | 1.99                         | 3.46 | 3.69 | 4.47 | 7.71 | 14.6 | 5.98 | .984                              | .959 | .949 | .934  | .805  | .462  | .849 |
| CAN (task 5)            |  | 2.17                         | 2.61 | 3.61 | 3.66 | 6.69 | 13.0 | 5.28 | .981                              | .977 | .951 | .956  | .851  | .552  | .878 |
| CAN (task 6)            |  | 2.09                         | 2.33 | 3.34 | 3.58 | 5.84 | 11.4 | 4.75 | .983                              | .982 | .959 | .958  | .883  | .638  | .900 |
| CAN (all tasks)         |  | 1.98                         | 4.58 | 6.91 | 3.54 | 4.01 | 12.1 | 5.52 | .985                              | .925 | .852 | .958  | .939  | .566  | .871 |
| <b>BREATH. RATE</b>     |  |                              |      |      |      |      |      |      |                                   |      |      |       |       |       |      |
| Methods                 |  | Root Mean Square Error / BPM |      |      |      |      |      |      | Pearson’s Correlation Coefficient |      |      |       |       |       |      |
|                         |  | 1                            | 2    | 3    | 4    | 5    | 6    | Avg. | 1                                 | 2    | 3    | 4     | 5     | 6     | Avg. |
| Tarassenko et al. [8]   |  | 4.84                         | 4.52 | 4.82 | 6.17 | 5.60 | 6.85 | 5.52 | .363                              | .452 | .299 | .197  | .192  | .071  | .294 |
| <b>OURS: Part. Dep.</b> |  |                              |      |      |      |      |      |      |                                   |      |      |       |       |       |      |
| Motion-only CNN         |  | 3.51                         | 4.15 | 5.07 | 4.73 | 4.78 | 6.17 | 4.74 | .530                              | .458 | .348 | .482  | .415  | .197  | .405 |
| Stacked CNN             |  | 3.15                         | 3.93 | 4.48 | 4.28 | 4.62 | 7.21 | 4.61 | .594                              | .490 | .422 | .531  | .489  | .125  | .442 |
| CAN                     |  | 3.10                         | 3.77 | 5.29 | 4.84 | 4.95 | 6.01 | 4.66 | .605                              | .516 | .351 | .452  | .450  | .237  | .435 |
| <b>OURS: Part. Ind.</b> |  |                              |      |      |      |      |      |      |                                   |      |      |       |       |       |      |
| Motion-only CNN         |  | 3.55                         | 4.50 | 6.42 | 6.35 | 6.55 | 6.06 | 5.57 | .559                              | .437 | .274 | .173  | .098  | .224  | .294 |
| Stacked CNN             |  | 3.93                         | 4.11 | 7.34 | 7.34 | 7.99 | 7.49 | 6.37 | .502                              | .529 | .136 | .031  | -.014 | .100  | .214 |
| CAN                     |  | 3.15                         | 3.70 | 6.68 | 6.52 | 5.65 | 6.54 | 5.37 | .642                              | .602 | .276 | .221  | .416  | .109  | .377 |
| CAN (task 1)            |  | 3.14                         | 3.73 | 8.54 | 9.25 | 8.08 | 5.82 | 6.43 | .642                              | .612 | .136 | -.106 | .112  | .216  | .269 |
| CAN (task 2)            |  | 2.92                         | 3.70 | 8.34 | 7.18 | 6.68 | 5.73 | 5.76 | .692                              | .602 | .124 | .256  | .160  | .228  | .344 |
| CAN (task 3)            |  | 3.58                         | 3.73 | 6.68 | 6.50 | 6.14 | 5.74 | 5.39 | .556                              | .598 | .276 | .238  | .357  | .259  | .381 |
| CAN (task 4)            |  | 3.76                         | 3.83 | 6.14 | 6.52 | 6.69 | 5.39 | 5.39 | .530                              | .582 | .286 | .221  | .132  | .311  | .344 |
| CAN (task 5)            |  | 3.55                         | 3.79 | 6.69 | 6.47 | 5.65 | 5.45 | 5.27 | .566                              | .595 | .251 | .309  | .416  | .333  | .411 |
| CAN (task 6)            |  | 4.20                         | 3.73 | 8.00 | 7.72 | 7.24 | 6.54 | 6.24 | .430                              | .601 | .190 | .088  | .095  | .109  | .252 |
| CAN (all tasks)         |  | 3.50                         | 6.97 | 5.58 | 4.09 | 7.04 | 5.30 | 5.41 | .592                              | .331 | .339 | .516  | .241  | .385  | .400 |

**Tulyakov et al. [9]:** The algorithm has five hyper-parameters  $\nu$ ,  $\gamma$ ,  $\mu$ ,  $\beta$  and  $\rho$ . In the paper, the authors selected four of them by cross-validation on a subset of the MMSE-HR dataset and showed their great generalization ability. Thus we directly used the same settings ( $\nu = 0.0357$ ,  $\gamma = 0.01$ ,  $\mu = 0.0011$  and  $\beta = 0.005$ ) in our implementation. However, the authors do not mention how they selected  $\rho$ . After trying several different numbers, we chose  $\rho = 0.05$  in all of our experiments. It is

Table 2: RGB Video II, MAHNOB-HCI and Infrared Video dataset results. (RMSE = Root Mean Square Error,  $r$  = Pearson’s Correlation Coefficient)

| DATASET                        |  | RGB VIDEO II |        | MANHOB-HCI |      |
|--------------------------------|--|--------------|--------|------------|------|
|                                |  | Heart Rate   |        | Heart Rate |      |
| Methods                        |  | RMSE /BPM    | $r$    | RMSE /BPM  | $r$  |
| Estepp et al. [5]              |  | 19.2         | -.0541 | -          | -    |
| McDuff et al. [7]              |  | 0.33         | .9995  | 13.6       | 0.36 |
| Balakrishnan et al. [1]        |  | 16.3         | .0530  | 21.0       | 0.11 |
| De Haan et al. [6]             |  | 0.39         | .9993  | 6.52       | 0.82 |
| Wang et al. [10]               |  | 0.33         | .9996  | -          | -    |
| Tulyakov et al. [9]            |  | 7.06         | .7571  | 6.23       | 0.83 |
| <b>OURS: Transfer Learning</b> |  |              |        |            |      |
| CAN                            |  | 0.26         | .9998  | 6.44       | 0.84 |

  

| DATASET                 |  | IR Video   |       |              |       |
|-------------------------|--|------------|-------|--------------|-------|
|                         |  | Heart Rate |       | Breath. Rate |       |
| Methods                 |  | RMSE /BPM  | $r$   | RMSE /BPM    | $r$   |
| Chen et al. [4]         |  | 2.75       | .9682 | 0.89         | .9740 |
| <b>OURS: Part. Ind.</b> |  |            |       |              |       |
| Motion-only CNN         |  | 5.20       | .8900 | 1.71         | .9049 |
| Stacked CNN             |  | 2.87       | .9635 | 0.33         | .9966 |
| CAN                     |  | 1.91       | .9844 | 0.31         | .9970 |

also worth mentioning that the algorithm was only tuned and tested on the MMSE-HR dataset and the MAHNOB-HCI dataset, neither of which includes subjects with large head rotations. Nevertheless, in Task 3 to 6 of our RGB Video I dataset, every subject has significant levels of head rotation, which explains why Tulyakov et al. [9] performs badly on these tasks.

## References

- [1] Guha Balakrishnan, Fredo Durand, and John Guttag. “Detecting pulse from head motions in video”. In: *IEEE Conference on Computer Vision and Pattern Recognition (CVPR)*. IEEE. 2013, pp. 3430–3437.
- [2] Tadas Baltrušaitis, Peter Robinson, and Louis-Philippe Morency. “Openface: an open source facial behavior analysis toolkit”. In: *IEEE Winter Conference on Applications of Computer Vision (WACV)*. IEEE. 2016, pp. 1–10.
- [3] Frédéric Bousefsaf, Choubeila Maaoui, and Alain Pruski. “Continuous wavelet filtering on webcam photoplethysmographic signals to remotely assess the instantaneous heart rate”. In: *Biomedical Signal Processing and Control* 8.6 (2013), pp. 568–574. ISSN: 17468094. DOI: 10.1016/j.bspc.2013.05.010.
- [4] Weixuan Chen, Javier Hernandez, and Rosalind W. Picard. “Non-contact physiological measurements from near-infrared video of the neck”. In: *arXiv preprint arXiv:1805.09511* (2017).
- [5] Justin R Estepp, Ethan B Blackford, and Christopher M Meier. “Recovering pulse rate during motion artifact with a multi-imager array for non-contact imaging photoplethysmography”. In: *IEEE International Conference on Systems, Man and Cybernetics (SMC)*. Vol. 940. IEEE. 2014, pp. 1462–1469.
- [6] Gerard de Haan and Vincent Jeanne. “Robust pulse rate from chrominance-based rPPG”. In: *IEEE Transactions on Biomedical Engineering* 60.10 (2013), pp. 2878–2886.
- [7] D McDuff, S Gontarek, and RW Picard. “Improvements in Remote Cardio-Pulmonary Measurement Using a Five Band Digital Camera.” In: *IEEE Transactions on Biomedical Engineering* 61.10 (2014), pp. 2593–2601.

- [8] L Tarassenko et al. “Non-contact video-based vital sign monitoring using ambient light and auto-regressive models”. In: *Physiological measurement* 35.5 (2014), p. 807.
- [9] Sergey Tulyakov et al. “Self-adaptive matrix completion for heart rate estimation from face videos under realistic conditions”. In: *IEEE Conference on Computer Vision and Pattern Recognition (CVPR)*. IEEE. 2016, pp. 2396–2404.
- [10] Wenjin Wang et al. “Algorithmic principles of remote PPG”. In: *IEEE Transactions on Biomedical Engineering* 64.7 (2017), pp. 1479–1491. DOI: 10.1109/TBME.2016.2609282.
